# Supplementary material for: HyKGE: A Hypothesis Knowledge Graph Enhanced Framework for Accurate and Reliable Medical LLMs Responses
Source: arXiv:2312.15883 source file (2024-04-19)
Supplement: Supplementary file 1 [file 7_Appendix.tex]

% \section{Experiment Details}
